# Supplementary material for: Causal Priors and Their Influence on Judgements of Causality in Visualized Data
Source: arXiv:2408.16077 source file (2024-08-28)
Supplement: Supplementary file 1 [file sec-appendix.tex]

The appendix shows the overall results distribution of our studies.
\autoref{fig:wordresults} is the results from Study 1 and \autoref{fig:chartresults} is for Study 2.

\begin{figure}[htbp]
\centering
\includegraphics[width=\columnwidth]{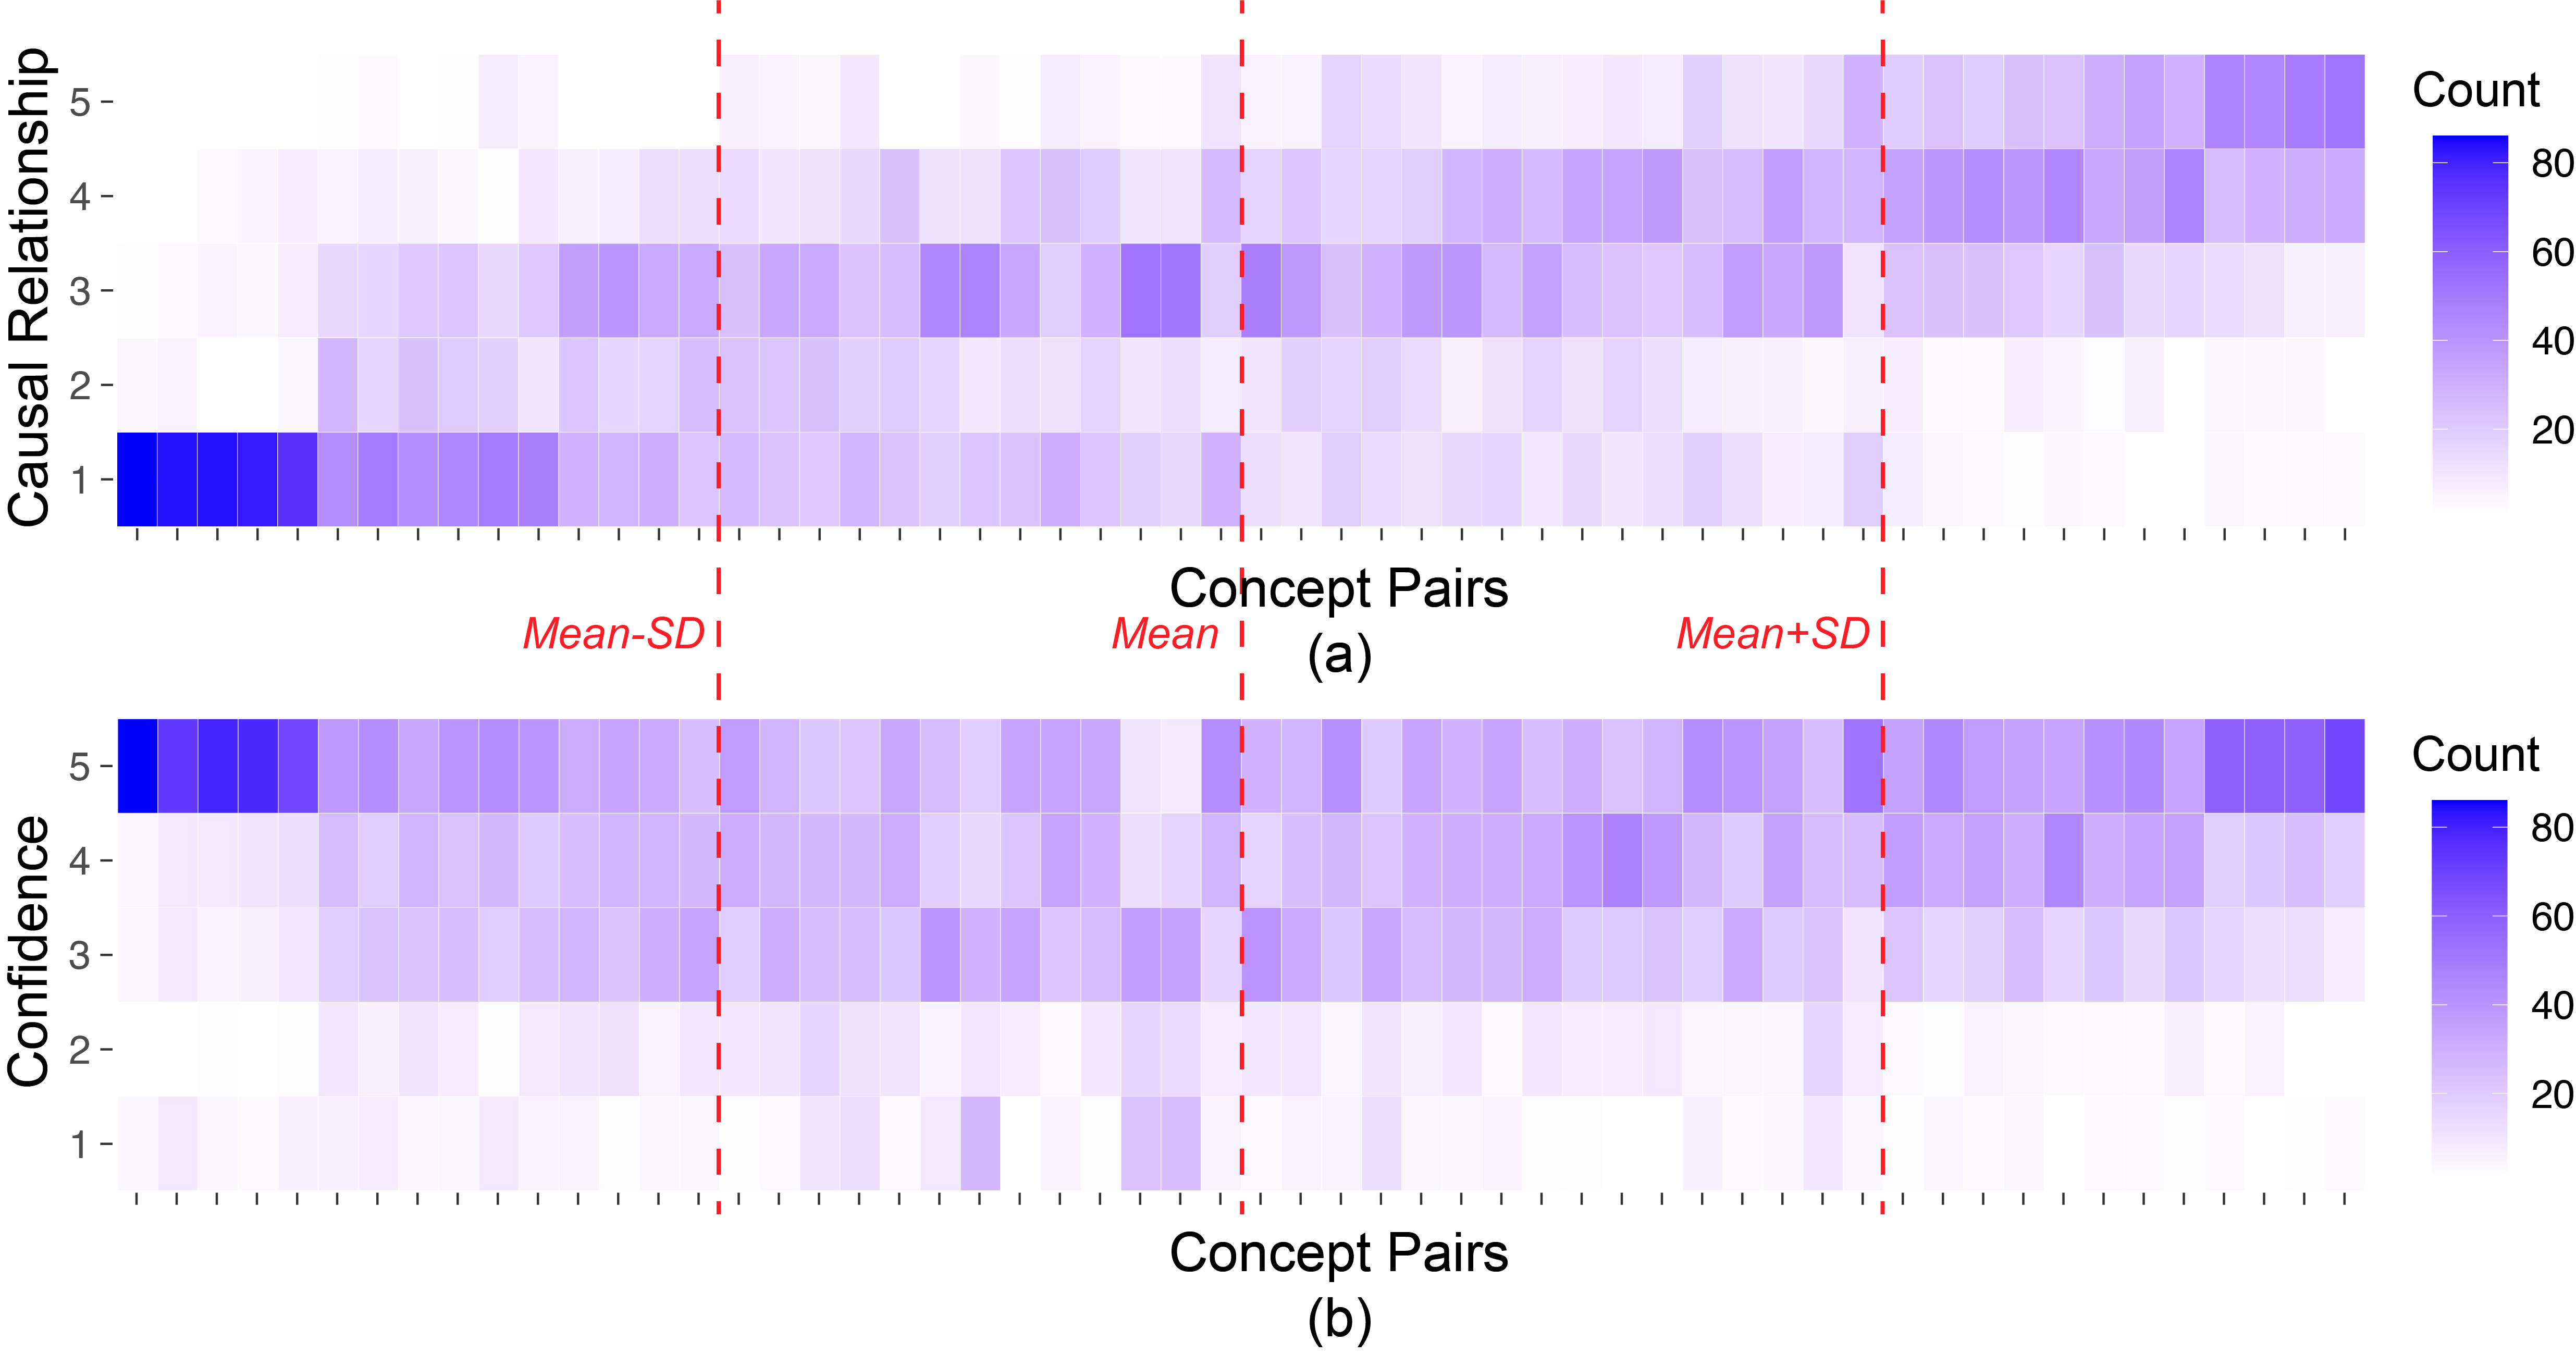}
\caption{ 
The detailed score distribution on the underlying prior for human cognition of causal inference in the collected dataset per causal relationship (a) and confidence (b) from our Study 1.
The concept pairs are ordered by increasing average causal relationship (causal prior), drawing \textcolor{red}{red} dashed lines with mean $\pm$ SD of causal relationships too (same as \autoref{fig:teaser}).
}
\label{fig:wordresults}
\end{figure}

\begin{figure}[htbp]
    \centering
    \includegraphics[width=\columnwidth]{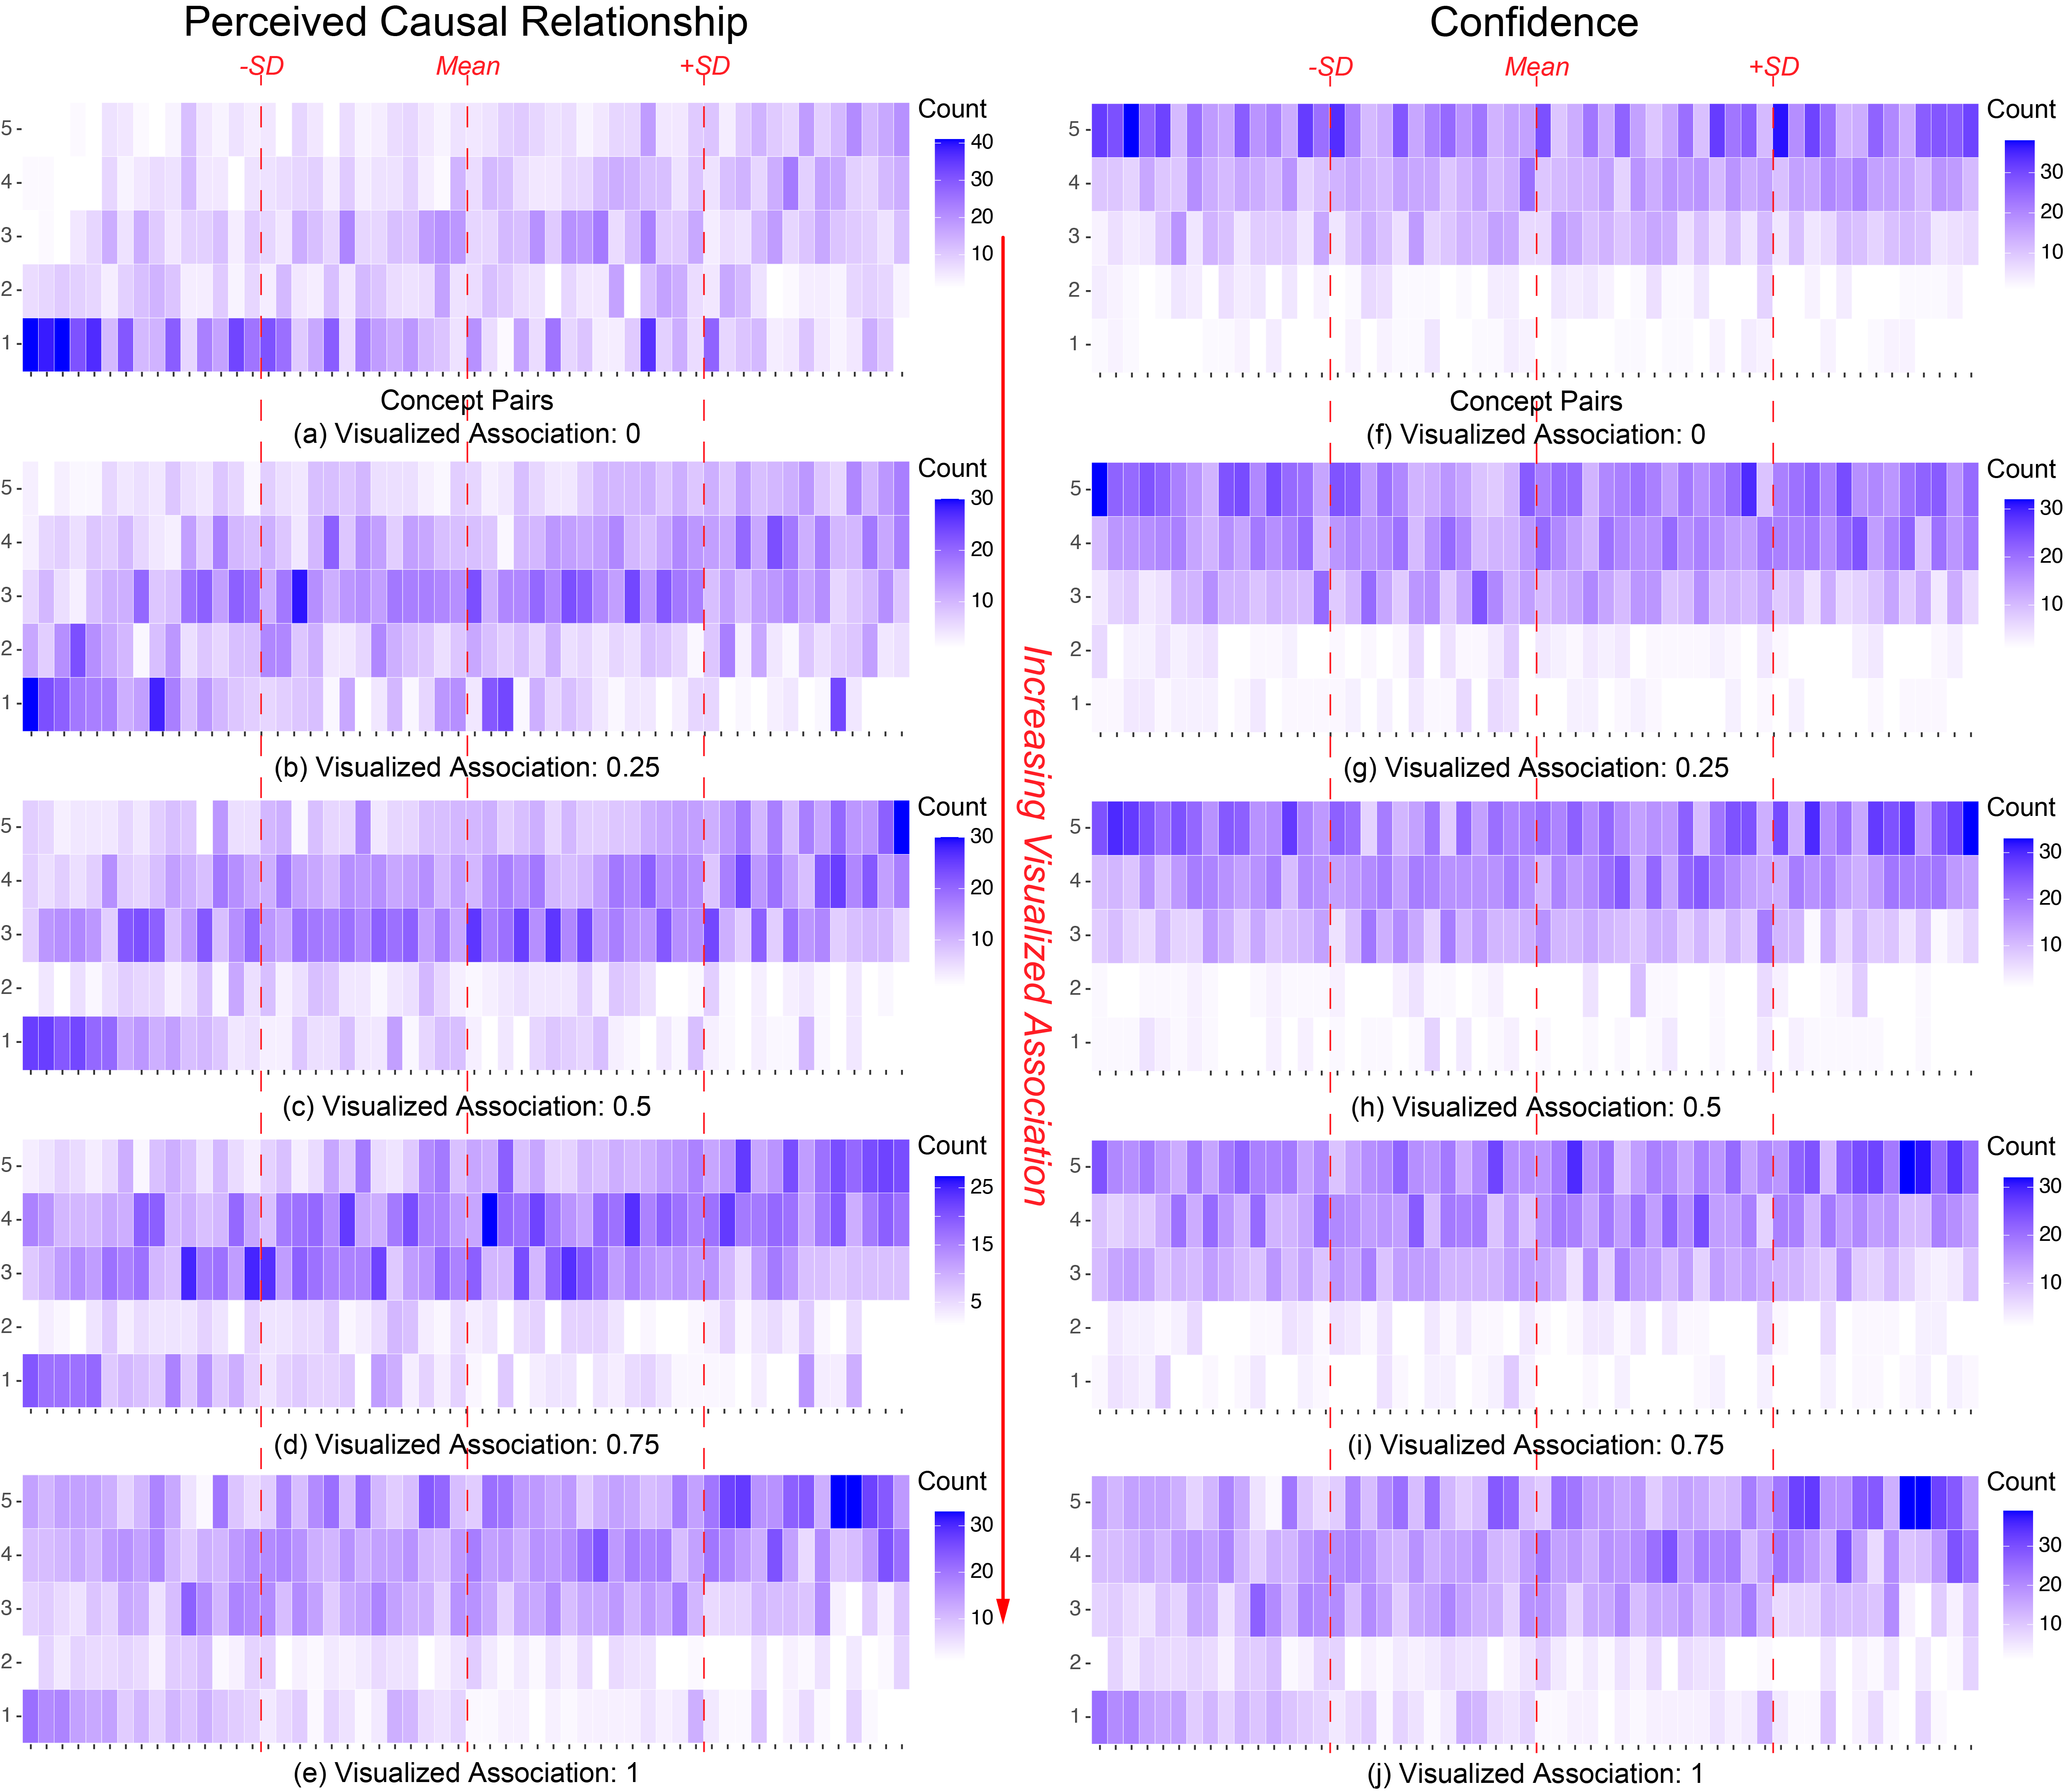}
    \caption{Our overall results from Study 2. The left column, (a) to (e), shows results per causal relationship while the right column, (f) to (j), shows corresponding confidence results respectively.
    The results consist of responses from 229 participants in Study 2. Each bin in a pair of charts (e.g., (a) and (f), (b) and (g)) consists of responses from around 50 users.
    From top to bottom, the visualized associations are gradually increased from 0 to 1. The concept pairs are ordered by increasing average causal relationship in Study 1, drawing \textcolor{red}{red} dashed lines with mean $\pm$ SD (same as \autoref{fig:teaser}). 
    }
    \label{fig:chartresults}
\end{figure}
